# Supplementary material for: MultiMUC: Multilingual Template Filling on MUC-4
Source: arXiv:2401.16209 source file (2024-01-29)
Supplement: Supplementary file 1 [file word_alignment.tex]

For word-to-word alignment using Awesome-align, we reused empirically-chosen hyperparameters from prior work for a similar task \cite{multicoref}: softmax normalization with probability thresholding of 0.001, 4 gradient accumulation steps, 1 training epoch with a learning rate of $2 \cdot 10^{-5}$, alignment layer of 16, and masked language modeling (``mlm''), translation language modeling (``tlm''), self-training objective (``so''), and parallel sentence identification (``psi'') training objectives. We additionally fine-tuned the resulting model, with the same hyperparameters, on 1200 English-Farsi, 2800 English-Chinese, and 2300 English-Arabic sentence pairs with gold word alignments, for 5 training epochs with a learning rate of $10^{-4}$ and ``so'' as the training objective.
